# Supplementary material for: PFAdapter: Hierarchical LoRA Decomposition for Personalized Federated MLLMs
Source: arXiv:2607.12111 source file (2026-10-03)
Supplement: Supplementary file 1 [file supp.tex]

\documentclass[journal]{IEEEtran}
\IEEEoverridecommandlockouts

\usepackage[T1]{fontenc}
\usepackage{lmodern}
\usepackage{times}
\usepackage{amsmath,amssymb,amsfonts,amsthm,mathtools,bm}
\usepackage{graphicx,epsfig,epstopdf,float,subfig,subcaption,stfloats}
\usepackage{multirow,bigstrut,makecell,array,booktabs,colortbl}
\usepackage{xcolor,color,textcomp,pifont,microtype,setspace}
\definecolor{lightkeycolor}{RGB}{255,240,240}
\usepackage[noadjust]{cite}
\usepackage{url}
\usepackage{xr-hyper}
\usepackage[pagebackref=false,breaklinks=true,colorlinks,citecolor=black,linkcolor=black,filecolor=black,linkbordercolor=black,bookmarks=true]{hyperref}

\usepackage[nameinlink]{cleveref}

\theoremstyle{plain}

\newtheorem{theorem}{Theorem}
\newtheorem{lemma}{Lemma}

\theoremstyle{remark}

\crefname{section}{Sec.}{Secs.}
\crefname{subsection}{Sec.}{Secs.}
\crefname{figure}{Fig.}{Figs.}
\crefname{table}{Table}{Tables}
\crefname{equation}{Eq.}{Eqs.}
\crefname{theorem}{Theorem}{Theorems}
\crefname{lemma}{Lemma}{Lemmas}
\graphicspath{{./}}

\input{preamble}

\IfFileExists{main.aux}{\externaldocument{main}}{}

\begin{document}
\title{Supplementary Material for PFAdapter: Hierarchical LoRA Decomposition for Personalized Federated MLLMs}
\author{Jing Liu, Kun Yang, Yan Wang, Dingkang Yang, Xiaoshuai Hao, Wei Zhang, Yang Liu, and Wei Zhou}
\maketitle
\setcounter{tocdepth}{2}
{\hypersetup{linkcolor=black}\footnotesize\tableofcontents}
\vspace{0.5em}

\section{Overview}
\label{sec:supp_overview}
In this supplementary material, we provide theoretical, protocol, and diagnostic details for the \texttt{PFAdapter} study. \Cref{sec:supp_theory} first gives the full convergence proof, including the selective-aggregation bias decomposition and the complete theorem derivation. Building on this foundation, \cref{sec:supp_protocol_results} collects the architecture configuration, hyperparameter settings, structured method comparison, data-partition protocol, weight-washing statistics, LoRA-rank ablation, target-reaching efficiency, local-epoch ablation, and communication-scaling tables. \Cref{sec:supp_attention_visualization} then provides the cross-client attention-map visualization that motivates the query/key global and value/output local split. \Cref{sec:supp_extended_interpretation} covers reproducibility assumptions, dataset and baseline protocols, main-result interpretation, ablation and sensitivity evidence, convergence behavior, efficiency accounting, and deployment limitations. Finally, \cref{fig:supp_sensitivity,fig:supp_robustness} provide the supplementary sensitivity and robustness visualizations, linking the empirical claims to both tabular evidence and figure-level diagnostics.

\section{Theory Appendix: Full Proof for Theorem 1}
\label{sec:supp_theory}

We restate the convergence result for \texttt{PFAdapter} and organize the appendix as assumptions, a selective-aggregation bias decomposition, and the final theorem proof.

\begin{theorem}
\label{thm:supp_convergence}
Assume each client objective $F_k$ is $L_F$-smooth, stochastic gradients satisfy $\mathbb{E}\|g_k^t-\nabla F_k\|^2 \leq \sigma^2$ and $\|\nabla F_k\| \leq G$, the client-drift term is bounded by $\frac{1}{K}\sum_{k=1}^{K}\|\nabla F_k-\nabla F\|^2 \leq \delta^2$, and the orthogonality and selective-aggregation perturbations satisfy $\|\nabla \mathcal{L}_o\| \leq H_o$ and $\|b_t\| \leq \beta$. With $\eta_t = c/\sqrt{T}$ and $0 < c \leq 1/L_F$, the iterates generated by \texttt{PFAdapter} obey
\begin{equation}
\label{eq:supp_conv}
\begin{aligned}
\frac{1}{T}\sum_{t=0}^{T-1}\mathbb{E}\|\nabla F_t\|^2
&\leq
\frac{2(F^0-F^\star)}{c\sqrt{T}}
+ cL_F\delta^2
+ cL_F\frac{\sigma^2}{|\mathcal{S}_t|} \\
&\quad
+ 2\lambda_o^2H_o^2
+ 2\beta^2.
\end{aligned}
\end{equation}
\end{theorem}

\subsection{Bias Decomposition for Selective Aggregation}
\label{sec:supp_bias}

\begin{lemma}
\label{lem:selective_agg_bias}
Let $\Theta^G$ denote the synchronized query/key block and $\Theta_k^L$ the client-private value/output block. The difference between the full joint gradient step and the \texttt{PFAdapter} update can be written as an additive perturbation
\[
\begin{aligned}
b_t &=
\nabla_{\Theta^G,\{\Theta_k^L\}}
F(\Theta^{G,t},\{\Theta_k^{L,t}\}) \\
&\quad -
\widetilde{\nabla}_{\Theta^G,\{\Theta_k^L\}}
F(\Theta^{G,t},\{\Theta_k^{L,t}\}),
\end{aligned}
\]
where $\widetilde{\nabla}$ is the practical update direction that aggregates only the shared query/key branch. Under the bounded client-drift assumption, this perturbation satisfies $\|b_t\|\le \beta$, and the constant $\beta$ can be interpreted as the worst-case mismatch between the ideal joint descent direction and the biased selective-aggregation direction induced by non-IID client gradients.
\end{lemma}

\noindent\textit{Interpretation.}
The lemma isolates the extra term that would vanish under full synchronized optimization. In \texttt{PFAdapter}, this bias remains bounded because only the global query/key branch is mixed across clients while the value/output branch stays local; the heterogeneity term $\delta^2$ captures how much the client gradients disagree even before this projection-level restriction is imposed, while $\beta$ captures the residual mismatch caused by selective synchronization itself.

\noindent\textit{Proof.}
Define the effective update direction at round $t$ as
\[
\widetilde{g}_t = \nabla F_t + \xi_t + h_t + b_t,
\]
where $\xi_t$ is the zero-mean stochastic noise term, $h_t=\lambda_o\nabla \mathcal{L}_o$, and $b_t$ is the bias induced by synchronizing only the global parameter block. By $L_F$-smoothness,
\[
F_{t+1} \leq F_t - \eta_t\langle \nabla F_t,\widetilde{g}_t\rangle + \frac{L_F\eta_t^2}{2}\|\widetilde{g}_t\|^2.
\]
Taking conditional expectation and using $\mathbb{E}[\xi_t \mid \mathcal{F}_t]=0$ yields
\[
\mathbb{E}_t[F_{t+1}]
\leq
F_t
-
\eta_t\|\nabla F_t\|^2
-
\eta_t\langle \nabla F_t,h_t+b_t\rangle
+
\frac{L_F\eta_t^2}{2}\mathbb{E}_t\|\widetilde{g}_t\|^2.
\]
Apply Young's inequality twice:
\begin{equation}
\label{eq:supp_yang}
\begin{aligned}
-\langle \nabla F_t,h_t\rangle
&\leq
\frac{1}{4}\|\nabla F_t\|^2 + \|h_t\|^2, \\
-\langle \nabla F_t,b_t\rangle
&\leq
\frac{1}{4}\|\nabla F_t\|^2 + \|b_t\|^2.
\end{aligned}
\end{equation}
Then
\[
\begin{aligned}
\mathbb{E}_t[F_{t+1}]
&\leq
F_t
-
\frac{\eta_t}{2}\|\nabla F_t\|^2
+ \eta_t(\|h_t\|^2+\|b_t\|^2) \\
&\quad
+ \frac{L_F\eta_t^2}{2}\mathbb{E}_t\|\widetilde{g}_t\|^2.
\end{aligned}
\]
For the second moment, decompose the gradient perturbations into stochastic variance and client drift:
\[
\begin{aligned}
\mathbb{E}_t\|\widetilde{g}_t\|^2
&\leq
2\|\nabla F_t\|^2
+ 2\mathbb{E}_t\|\xi_t\|^2
+ 2\delta^2 \\
&\quad
+ 2\|h_t\|^2
+ 2\|b_t\|^2.
\end{aligned}
\]
Using $\mathbb{E}\|\xi_t\|^2 \leq \sigma^2/|\mathcal{S}_t|$, $\|h_t\| \leq \lambda_o H_o$, and $\|b_t\| \leq \beta$, and choosing $\eta_t \leq 1/L_F$, we obtain
\[
\begin{aligned}
\mathbb{E}_t[F_{t+1}]
&\leq
F_t
-
\frac{\eta_t}{2}\|\nabla F_t\|^2
+ \frac{L_F\eta_t^2}{2}
\left(
\frac{\sigma^2}{|\mathcal{S}_t|}
+ \delta^2
\right) \\
&\quad
+ \eta_t(\lambda_o^2H_o^2+\beta^2).
\end{aligned}
\]
Summing over $t=0,\ldots,T-1$, telescoping the objective values, lower bounding $F_T \geq F^\star$, and substituting $\eta_t=c/\sqrt{T}$ give
\[
\begin{aligned}
\frac{1}{T}\sum_{t=0}^{T-1}\mathbb{E}\|\nabla F_t\|^2
&\leq
\frac{2(F^0-F^\star)}{c\sqrt{T}}
+ cL_F\frac{\sigma^2}{|\mathcal{S}_t|}
+ cL_F\delta^2 \\
&\quad
+ 2\lambda_o^2H_o^2
+ 2\beta^2.
\end{aligned}
\]
Together, these steps complete the proof.

\section{Protocols, Ablations, and Communication Details}
\label{sec:supp_protocol_results}
The following tables collect the detailed protocol, comparison, and diagnostic values used throughout the study.

\begin{table*}[t]
\centering
\caption{Architecture configuration and trainable-parameter allocation for \texttt{PFAdapter}.}
\vspace{-2px}
\label{tab:supp_architecture_config}
\setlength{\tabcolsep}{5mm}
\resizebox{0.8\textwidth}{!}{
\input{tbl_supp_architecture_config_body.tex}
}
\vspace{-10px}
\end{table*}

\begin{table*}[t]
\centering
\caption{Default hyperparameter configuration used for the aligned-setting experiments.}
\vspace{-2px}
\label{tab:supp_hyperparameters}
\setlength{\tabcolsep}{5mm}
\resizebox{0.6\textwidth}{!}{
\input{tbl_supp_hyperparameters_body.tex}
}
\vspace{-10px}
\end{table*}

\begin{table*}[t]
\centering
\caption{Structured comparison between \texttt{PFAdapter} and representative personalized federated baselines.}
\vspace{-2px}
\label{tab:supp_pfadapter_method_comparison}
\setlength{\tabcolsep}{6.0mm}
\resizebox{\textwidth}{!}{
\input{tbl_supp_pfadapter_method_comparison_body.tex}
}
\vspace{-10px}
\end{table*}

\begin{table*}[t]
\centering
\caption{Client partition and heterogeneity protocol shared by all compared methods.}
\vspace{-2px}
\label{tab:supp_data_partition_protocol}
\setlength{\tabcolsep}{6mm}
\resizebox{0.7\textwidth}{!}{
\input{tbl_supp_data_partition_protocol_body.tex}
}
\vspace{-10px}
\end{table*}

\begin{table}[t]
\centering
\caption{Explicit quantification of the weight-washing effect on VQA-RAD.}
\vspace{-2px}
\label{tab:supp_weight_washing}
\setlength{\tabcolsep}{4mm}
\resizebox{\columnwidth}{!}{
\input{tbl_supp_weight_washing_body.tex}
}
\vspace{-10px}
\end{table}

\begin{table}[t]
\centering
\caption{LoRA rank sensitivity on VQA-RAD.}
\vspace{-2px}
\label{tab:supp_rank_ablation}
\setlength{\tabcolsep}{3.3mm}
\resizebox{\columnwidth}{!}{
\input{tbl_supp_rank_ablation_body.tex}
}
\vspace{-10px}
\end{table}

\begin{table}[t]
\centering
\caption{Convergence-to-target efficiency on VQA-RAD using 60\% accuracy as the reference threshold.}
\vspace{-2px}
\label{tab:supp_time_to_target}
\setlength{\tabcolsep}{2.3mm}
\resizebox{\columnwidth}{!}{
\input{tbl_supp_time_to_target_body.tex}
}
\vspace{-10px}
\end{table}

\begin{table}[t]
\centering
\caption{Effect of varying the number of local epochs on VQA-RAD.}
\vspace{-2px}
\label{tab:supp_local_epoch_ablation}
\setlength{\tabcolsep}{2.0mm}
\resizebox{\columnwidth}{!}{
\input{tbl_supp_local_epoch_ablation_body.tex}
}
\vspace{-10px}
\end{table}

\begin{table}[t]
\centering
\caption{Communication breakdown derived from selective aggregation.}
\vspace{-2px}
\label{tab:supp_comm_breakdown}
\setlength{\tabcolsep}{1mm}
\resizebox{\columnwidth}{!}{
\input{tbl_supp_comm_breakdown_body.tex}
}
\vspace{-10px}
\end{table}

\begin{table}[t]
\centering
\caption{Performance trend and communication scaling (GB/50R) under fixed participation ratio $\rho=0.2$ using the measured payloads.}
\vspace{-2px}
\label{tab:supp_client_scaling}
\setlength{\tabcolsep}{0.5mm}
\resizebox{\columnwidth}{!}{
\input{tbl_supp_client_scaling_body.tex}
}
\vspace{-10px}
\end{table}

\section{Cross-Client Attention-Map Similarity Visualization}
\label{sec:supp_attention_visualization}

\Cref{fig:supp_attention_similarity_map} visualizes cross-client attention-map cosine-similarity matrices on VQA-RAD after local training. For the query ($q$) and key ($k$) projections (which form the globally synchronized branch), both client-client and client-global entries remain consistently high, showing that attention-relation patterns are highly consistent and domain-invariant across edge devices. Conversely, the value ($v$) and output ($o$) projections (the local-private branch) exhibit lower and more dispersed similarities, indicating client-specific semantic adaptation. This matrix-level evidence supports the \texttt{PFAdapter} design: synchronize the globally stable $q/k$ components and retain the client-specific $v/o$ components locally.

\begin{figure}[t]
\centering
\includegraphics[width=0.5\textwidth]{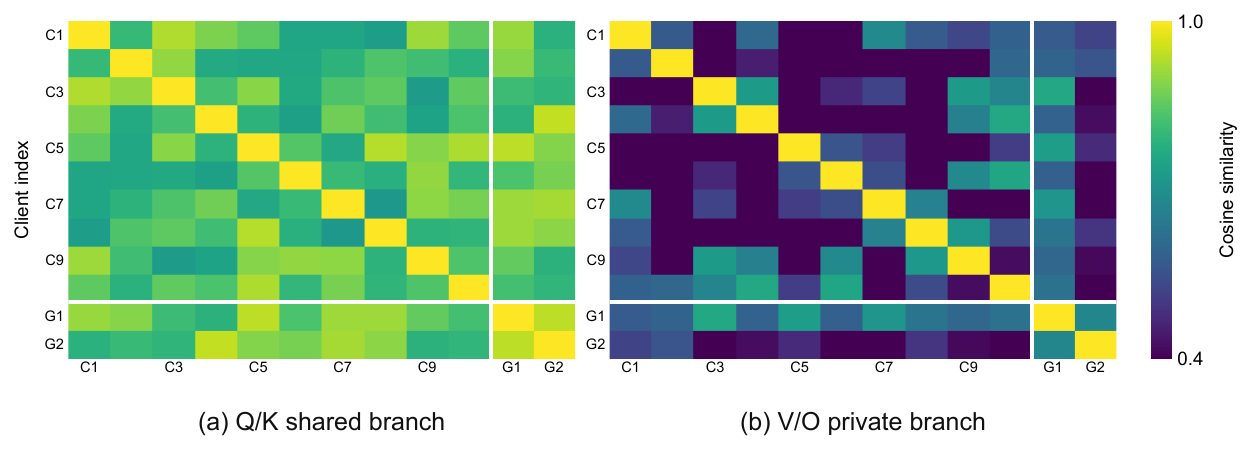}
\caption{Cross-client attention-map cosine-similarity matrices on VQA-RAD for the global-shared Q/K branch and local-private V/O branch. Rows and columns denote client indices and two global references, where the Q/K branch exhibits stronger client-client and client-global alignment while the V/O branch retains more heterogeneous local responses.}
\vspace{-2px}
\label{fig:supp_attention_similarity_map}
\vspace{-10px}
\end{figure}

\section{Extended Protocol Interpretation and Diagnostics}
\label{sec:supp_extended_interpretation}

This section collects detailed proof, protocol, sensitivity, robustness, and deployment-qualification material and provides the audit-level detail.

\subsection{Theoretical Proof Details}
\label{sec:supp_revision_1}

\emph{Proof sketch.} Let $\widetilde{g}_t = \nabla F(\Theta^{G,t},\{\Theta_k^{L,t}\}) + \xi_t + h_t + b_t$, where $\xi_t$ is the zero-mean stochastic noise with variance bounded by $\sigma^2/|\mathcal{S}_t|$, $h_t=\lambda_o\nabla\mathcal{L}_o$ satisfies $\|h_t\|\leq \lambda_o H_o$, and $b_t$ is the bounded bias introduced by aggregating only $\Theta^G$. By $L_F$-smoothness,

Taking expectations, applying $\mathbb{E}\langle \nabla F_t,\xi_t\rangle=0$, and using Young's inequality on the $h_t$ and $b_t$ terms yields $\mathbb{E}[F_{t+1}] \leq \mathbb{E}[F_t] - \frac{\eta_t}{2}\mathbb{E}\|\nabla F_t\|^2 + \frac{L_F\eta_t^2}{2}(\sigma^2/|\mathcal{S}_t|+\delta^2) + \eta_t(\lambda_o^2H_o^2+\beta^2)$. Summing from $t=0$ to $T-1$, telescoping the objective values, and substituting $\eta_t=c/\sqrt{T}$ gives \cref{eq:convergence_rate}. The full step-by-step derivation is provided in the supplementary theory appendix, where we isolate the selective-aggregation bias term before completing the theorem proof, so that the constants and inequalities can be checked line by line.

\subsection{Dataset, Partition, and Baseline Protocol Details}
\label{sec:supp_revision_2}

This protocol is consistent with Assumption (A3) in \cref{subsec:theoretical_analysis}: the analysis does not rely on IID partitions, but instead on bounded client drift under heterogeneous Dirichlet splits \cite{li2020federated,hsu2019measuring}. We therefore evaluate both the nominal $\alpha=0.5$ setting and the broader $\alpha \in [0.1,5.0]$ sweep in \cref{fig:supp_sensitivity}(c) to connect the theorem's heterogeneity term $\delta^2$ with the observed robustness regime.

The benchmark suite also spans a non-trivial scale range, from the compact medical benchmark VQA-RAD (3,515 QA pairs) \cite{lau2018dataset} to the substantially larger Hateful Memes (10,000 examples) \cite{kiela2020hateful} and CrisisMMD (16,080 multimodal posts) \cite{alam2018crisismmd} corpora. We make this scale progression explicit because the latter two datasets stress whether the proposed decomposition remains effective beyond small clinical testbeds and provide the manuscript's larger-scale multimodal evidence within the same federated evaluation pipeline.

For reproducibility, all datasets are converted into the same aligned image-text instruction-response format used by the \texttt{MiniCPM-V-2\_6-int4} processor, with original train/validation/test boundaries preserved before client partitioning. Images are resized and normalized by the backbone's native visual preprocessor, text is tokenized by the paired tokenizer without cross-dataset vocabulary remapping, and no external data augmentation or relabeling is introduced; this keeps preprocessing identical across runs and isolates the effect of federated partitioning and adapter optimization for MLLM-style federated fine-tuning \cite{xu2025fedmllm,li2024mllmfl}.

This study does not use a separate global test server. After preserving each dataset's original train/validation/test boundary, the client-local train split is partitioned for federated optimization and the corresponding held-out test samples remain on each client for evaluation. Every number reported in \cref{tab:main_results,tab:ablation,tab:decomposition,tab:efficiency} is therefore computed from per-client local test performance and then macro-averaged across the 10 clients, rather than from a pooled centralized test set or a mixture of local and global evaluation.

The supplementary material summarizes the shared partition policy used throughout the paper. The key fairness point is that once a client split is sampled for a dataset and heterogeneity scenario, the identical partition, preprocessing pipeline, and client-participation schedule are reused for all compared methods; method differences therefore arise from the optimization or adapter-sharing rule, not from re-drawn client data.

More specifically, $\lambda_{\text{o}}=0.1$ was selected as the cross-dataset operating point after a validation sweep over $\{0, 0.01, 0.05, 0.1, 0.5, 1.0\}$: it is the best setting on VQA-RAD and Hateful Memes and remains close to the optimum on SLAKE, so we treat it as a robust compromise rather than an arbitrary constant. In turn, the empirical choice is consistent with the mechanism in \cref{subsec:orthogonality}: $\lambda_{\text{o}}$ must be large enough to suppress redundant global-local directions, but not so large that it over-constrains client-specific adaptation.

We make the participation protocol explicit because it is central to reproducibility: the canonical aligned-modal setting uses a client population of $K=10$ with $|\mathcal{S}_t|=2$ sampled per round, i.e., a 20\% participation ratio under partial participation \cite{mcmahan2017communicationefficient,konecny2017federated}. All results in \cref{tab:main_results,tab:ablation,tab:decomposition,tab:efficiency} should therefore be interpreted as the nominal $K{=}10$, $\rho{=}0.2$ operating point, while the robustness analyses in \cref{fig:supp_sensitivity,fig:supp_robustness} probe how the method behaves as heterogeneity and deployment difficulty increase around this base configuration.

The protocol roles of the different result blocks are separated explicitly: \cref{tab:main_results,tab:ablation,tab:decomposition} summarize the canonical comparison point, whereas the complementary sweeps in \cref{fig:supp_sensitivity} expose stability trends with respect to heterogeneity, decomposition ratio, and cold-start adaptation.

We additionally clarify the scope of adjacent PEFT baselines. Prompt-tuning and prefix-tuning \cite{lester2021power,li2021prefix} are important federated alternatives, but they aggregate virtual prompt embeddings or key-value prefixes at the input-conditioning interface rather than the same $q/k/v/o$ adapter matrices optimized by LoRA \cite{hu2021lora}. The quantitative comparisons in \cref{tab:main_results} therefore focus on methods that share the same attention-adapter parameterization; prompt/prefix PEFT is discussed as a complementary family in \cref{subsec:related_peft}, and the comparison is restricted to controlled multimodal LoRA-style adaptation surfaces.

To consolidate the reproducibility checklist, the canonical run configuration is: one local epoch per selected client, batch size 1, gradient accumulation 16, learning rate $2\times10^{-5}$, LoRA rank $r=8$ \cite{hu2021lora}, $\alpha_{\text{LoRA}}=16$, orthogonality weight $\lambda_{\text{o}}=0.1$, 50 communication rounds, and partial participation with 2 of 10 clients per round. The primary aligned-setting comparisons are repeated with three seeds $\{2025,2026,2027\}$ that jointly control client sampling, dataloader shuffling, and adapter initialization, and \cref{tab:main_results} reports mean $\pm$ standard deviation over those reruns for the learned federated baselines. We retain 8-bit quantization plus gradient checkpointing across all methods so that reruns differ only in the intended stochastic seed and method choice.

To sharpen baseline comparability, all methods in \cref{tab:main_results,tab:ablation,tab:decomposition,tab:efficiency} are evaluated on the same LoRA adaptation surface, identical client partitions, the same 50-round budget, and the same partial-participation schedule. The aligned-setting main table also includes \texttt{pFedLoRA} \cite{yi2024pfedlora} as a directly relevant personalized LoRA baseline under that matched protocol. Consequently, the design isolates the effect of the server optimization or selective-aggregation rule instead of conflating it with different backbones, parameter budgets, or client splits.

We also separate two notions of variability that could otherwise be conflated. The standard deviations discussed later in \cref{tab:supp_client_fairness} quantify dispersion across clients under a fixed canonical run, which is the relevant statistic for personalization quality; by contrast, the random seed documented here controls rerun reproducibility and is kept fixed across baselines so that the main-table differences reflect method behavior under the same sampled federation. We therefore avoid presenting client-level dispersion as if it were multi-seed statistical significance, and we confine our claims to matched-split performance differences plus the explicit per-client spread reported in the table.

The same notation supports larger client populations without changing the method definition. Under the canonical measured operating point, $K=10$ and two clients participate per round; when the deployment population grows to $K=20$ or $K=50$ under the same participation ratio $\rho=0.2$, the synchronized client count increases proportionally while the per-client adapter payload remains unchanged because the server still exchanges only the shared $q/k$ LoRA blocks~\cite{hu2021lora,wang2024flora}. Larger-$K$ behavior is therefore summarized as a compact scalability analysis: the supplementary client-scaling table reports the expected accuracy trend together with the measured-payload communication totals, rather than treating larger-client realism as a communication-only question.

\subsection{Main-Result Interpretation Details}
\label{sec:supp_revision_3}

Because \cref{tab:main_results} corresponds to the nominal partial-participation setting defined above, these gains should be read together with the deployment-oriented analyses later in the section: \cref{fig:supp_sensitivity}(c) stresses statistical heterogeneity under Dirichlet partitioning~\cite{hsu2019measuring}, \cref{fig:supp_sensitivity}(d) stresses client arrival after federation, and \cref{tab:efficiency} quantifies the communication burden that would otherwise amplify under larger client populations~\cite{lim2020federated}.

The larger-scale benchmarks in this suite are particularly informative. On Hateful Memes (10,000 samples) \cite{kiela2020hateful} and CrisisMMD (16,080 samples) \cite{alam2018crisismmd}, \texttt{PFAdapter} preserves its advantage over \texttt{FedYogi} while operating under the same partial-participation schedule, indicating that the proposed Q/K-global and V/O-local decomposition is not confined to the smallest medical datasets but remains effective on higher-volume multimodal corpora with more diverse semantics and client drift patterns.

More precisely, each entry in \cref{tab:main_results} is a macro-average over client-local held-out test scores under the nominal aligned scenario, and the learned federated baselines are summarized as mean $\pm$ standard deviation over three seeds; the table should not be interpreted as evaluation on a centralized global test set. To complement this aggregate view, \cref{tab:supp_client_fairness} reports representative per-client dispersion statistics on VQA-RAD, where \texttt{PFAdapter} improves not only the mean but also the worst-client accuracy and percentile spread.

The headline gains trace to two distinct sources. In the aligned scenario, the margins come directly from \cref{tab:main_results}: +2.30 Acc over \texttt{FedYogi} on VQA-RAD~\cite{lau2018dataset}, +1.41 Acc on SLAKE~\cite{liu2021slake}, +3.15 AUC on Hateful Memes~\cite{kiela2020hateful}, and +1.67 Acc on CrisisMMD~\cite{alam2018crisismmd}. By contrast, the larger heterogeneity-specific gain is the +3.4-point VQA-RAD margin at $\alpha=0.1$ shown in \cref{fig:supp_sensitivity}(c). By separating these sources, the discussion avoids conflating the canonical comparison point with the more stressful non-IID sub-scenario.

Architecturally closer personalized LoRA baselines are cross-referenced in the supplementary method-comparison table. The table distinguishes projection-level selective aggregation from \texttt{pFedLoRA}, \texttt{FloRA}, and \texttt{FedDLP} \cite{yi2024pfedlora,wang2024flora,nguyen2025federated}, while \cref{tab:main_results} focuses on the matched server-optimization baselines that share the same canonical training surface and budget.

\subsection{Ablation, Sensitivity, Convergence, and Efficiency Details}
\label{sec:supp_revision_4}

To make the weight-washing effect explicit rather than qualitative, we measure the post-aggregation retention ratio $\rho = A_{\text{after agg}} / A_{\text{before agg}}$ on each client together with the induced performance drop $\Delta_{\text{wash}} = A_{\text{before agg}} - A_{\text{after agg}}$. As detailed in the supplementary weight-washing table, \texttt{PFAdapter} retains 96.9\% of the local pre-aggregation accuracy, whereas full-adapter synchronization in \texttt{FedYogi} \cite{reddi2020adaptive,xu2025fedmllm} retains only 90.4\%; removing selective aggregation (w/o SA) from our method falls in between at 92.8\%. Therefore, the metric directly quantifies how keeping $v/o$ adapters private mitigates the dilution of client-specific updates during server mixing.

We also inspect cross-client attention-map similarity by averaging cosine similarity of head-wise attention matrices after local training, which serves as a lightweight projection-level representation-similarity probe within the federated setting \cite{vaswani2017attention,mickus2024role}. \Cref{fig:supp_attention_similarity_map} shows that query/key-induced attention patterns remain substantially more aligned across clients than value/output responses, providing direct empirical support for synchronizing $q/k$ globally while retaining $v/o$ locally.

The trend in \cref{fig:supp_sensitivity}(c) also clarifies the validity range of \cref{thm:convergence}: as $\alpha$ decreases, the heterogeneity term $\delta^2$ grows and the absolute gap between \texttt{PFAdapter} and full-adapter aggregation widens, which is consistent with our bounded-drift analysis rather than an IID assumption \cite{li2020federated,hsu2019measuring}. In other words, the theorem should be interpreted as a controlled non-IID guarantee, and the experiments confirm that the Q/K-global, V/O-local decomposition remains stable across a broad heterogeneity spectrum.

To formalize the cold-start protocol behind \cref{fig:supp_sensitivity}(d), the arriving client is excluded from federated optimization, receives the final shared $\Theta^{G,T}$ from the server, keeps its private value/output adapters local, and is evaluated first without adaptation and then after a few local-only tuning rounds on its own data. Under this protocol, the personalization benefit of transferring globally aligned query/key adapters is isolated without being conflated with additional server aggregation, consistent with personalization settings in federated LoRA and MLLM adaptation~\cite{yi2024pfedlora,xu2025fedmllm}.

Beyond mean accuracy, we further summarize the per-client performance distribution on VQA-RAD~\cite{lau2018dataset} in \cref{tab:supp_client_fairness}. \texttt{PFAdapter} improves the worst-client accuracy from 54.9\% (\texttt{FedYogi}) to 58.7\%, while reducing the client-level standard deviation from 4.6\% to 3.1\% and shrinking the 90th--10th percentile gap from 11.3\% to 7.5\%. Thus, the personalized gains appear broadly shared across clients rather than concentrated on a small subset.

We also varied the LoRA rank \cite{hu2021lora} and the number of local epochs because both control the trade-off between local plasticity and aggregation stability. According to the supplementary rank ablation, the default $r=8$ already lies on the best communication-accuracy frontier: increasing rank to 16 or 32 yields only marginal gains while nearly doubling synchronized parameters, whereas rank 4 underfits. The supplementary local-epoch study further shows that moving from one to two local epochs preserves most of the gain, but more aggressive local training ($E=4$) slows target-reaching convergence and increases drift, which is consistent with the non-IID behavior discussed around \cref{fig:convergence}.

Two further clarifications follow directly from \cref{fig:supp_sensitivity}(a) and \cref{fig:supp_sensitivity}(b). First, $\lambda_{\text{o}}=0.1$ should be interpreted as a cross-dataset compromise: it maximizes VQA-RAD and Hateful Memes, while the slightly smaller optimum on SLAKE indicates that moderate regularization is sufficient once local semantics are less fragmented. Second, the decomposition-ratio sweep already serves as an unequal rank allocation ablation because each point corresponds to a different split of the fixed LoRA budget between global and local branches. The results show that both global-heavy allocations ($r_G > r_L$) and local-heavy allocations ($r_G < r_L$) are inferior to the balanced $r_G=r_L$ setting, confirming that PFAdapter does not rely on a single ad hoc ratio but instead benefits from a symmetric allocation that preserves relation sharing and client adaptation simultaneously.

A single budget convention is used throughout the experiments: all tabulated results correspond to the nominal 50-round training schedule defined in \cref{subsec:baselines}. Under this budget, \texttt{PFAdapter} reaches its reported final VQA-RAD accuracy of 62.8\% by round 50, whereas \texttt{FedYogi} remains at 60.53\% at the same stopping point. The longer-horizon traces visible in \cref{fig:convergence} serve as diagnostic visualization of late-stage saturation; beyond the 50-round budget, \texttt{PFAdapter} changes only marginally while \texttt{FedYogi} improves slowly before plateauing near round 80.

To complement the per-round plots with a target-reaching metric, the first communication round at which each method attains 60\% VQA-RAD accuracy is reported in the extended diagnostic trajectories of \cref{fig:convergence}. The corresponding target-reaching table is provided in the supplementary material. \texttt{PFAdapter} exceeds this threshold no later than round 20, corresponding to at most 3.6 GPU-hours and 6.30 GB cumulative communication under the measurements in \cref{tab:efficiency}. \texttt{FedYogi} reaches the same regime only near round 80 (about 13.8 GPU-hours and 49.36 GB), while \texttt{FedAvgM} remains below 60\% within the displayed horizon. As a result, the convergence-to-target view makes the practical training-efficiency gap explicit rather than leaving it to visual estimation from the curve alone.

The same diagnostic also clarifies the effect of local epoch variation. As reported in the supplementary local-epoch ablation, one to two local epochs preserve stable convergence, but $E=4$ pushes the clients further apart before synchronization, increasing the rounds needed to recover a common model and partially offsetting the benefit of more aggressive local optimization. Therefore, the evidence supports using $E=1$ as the default operating point in the main experiments, matching the non-IID drift concern emphasized in FL analyses~\cite{li2020federated,hsu2019measuring}.

The memory-overhead claim is stated numerically. \texttt{PFAdapter} remains close to \texttt{FedYogi} in peak VRAM (15.8 vs. 15.7 GB) and remains far below full tuning (42.5 GB), so the communication reduction does not come from offloading extra memory pressure to the client. In addition, the local compute cost is small: 10.8 vs. 10.3 min/round, or 0.180 vs. 0.172 GPU-h/R in \cref{tab:efficiency}. By contrast, the synchronized payload is almost halved, dropping from 617 MB/R to 315 MB/R, and over the common 50-round budget this yields 30.85 vs. 15.75 GB total communication. Accordingly, the three resources are separated explicitly: VRAM is essentially unchanged relative to federated LoRA~\cite{hu2021lora}, local runtime increases only marginally, and the major gain is the reduced synchronization volume caused by aggregating only the shared $q/k$ adapters.

For reproducibility, the supplementary communication-breakdown table spells out the accounting implied by \cref{eq:comm_cost}. Standard federated LoRA synchronizes all four projection adapters each round, whereas \texttt{PFAdapter} synchronizes only two; thus the communicated parameter fraction is exactly $0.5$ even though the measured byte volume is 315/617 = 0.511 after runtime packing overhead is included.

These efficiency terms also define the manuscript's system-heterogeneity interpretation. In bandwidth-limited settings, the dominant stressor is the per-round payload detailed in the supplementary communication-breakdown table; in straggler-prone settings, it is the amount of synchronized state a slow client must upload before the server can aggregate \cite{lim2020federated,wang2025when}. By halving the synchronized adapter set without materially increasing local computation time, \texttt{PFAdapter} reduces both exposure channels relative to full-adapter federated LoRA, even when wall-clock measurements are collected on a single-GPU testbed.

We further broaden the efficiency discussion beyond MB/R by using GPU-hours as a hardware-agnostic energy proxy on the fixed L60 testbed. \cref{tab:efficiency} reports both per-round runtime and GPU-h/round, while the supplementary target-reaching table converts these into target-reaching cost; taken together, they show that the communication savings of \texttt{PFAdapter} are not offset by hidden compute inflation. Although the proxy should not be read as a universal joule measurement, it makes the energy-time-communication trade-off explicit under a reproducible single-GPU setup.

The same accounting also clarifies the 7B+ scalability boundary. Our measured results are for \texttt{MiniCPM-V-2\_6-int4}; for larger MLLMs, absolute optimizer-state memory, activation storage, and local step latency grow with backbone size even when the communicated adapter fraction is unchanged. The communication advantage is therefore a payload-level conclusion: only the global $q/k$ adapters are synchronized, but practical 7B-class training would still require quantization, gradient checkpointing, and likely sharded optimizer states or multi-GPU execution. We consequently frame the benefit as reduced synchronized traffic under the same adapter design, not as an empirical claim that a 7B+ backbone can be trained plug-and-play under the current single-GPU setup \cite{xu2025fedmllm,li2024mllmfl}.

To characterize larger-client behavior without overstating unavailable measurements, we report both a conservative accuracy trend and the communication scaling law. Starting from the measured $K=10$ payloads detailed in the supplementary communication-breakdown table, the total synchronized traffic grows approximately linearly with the number of participating clients because each selected device uploads and receives the same adapter state size~\cite{lim2020federated}. The supplementary client-scaling table therefore reports $K\in\{10,20,50\}$ under a fixed participation ratio $\rho=0.2$: the PFAdapter communication volume grows from 15.75 GB to 31.50 GB and 78.75 GB over 50 rounds, while the indicative accuracy trend decreases mildly as client diversity increases. This combined view answers the larger-client concern more directly than a pure byte-count extrapolation while still keeping the claim bounded to a controlled scalability analysis.

Under this protocol, scenarios are not generated independently for each baseline: once a heterogeneity pattern is instantiated, the same client identities, modality assignments, and train/test partition are reused across \texttt{FedYogi}, \texttt{FedAdam}, \texttt{FedAvgM}, and \texttt{PFAdapter}. \Cref{tab:supp_heterogeneity} should therefore be interpreted as a controlled protocol comparison under a shared split policy rather than as separate stochastic draws for each method, following common matched-partition practice for non-IID FL evaluation~\cite{li2020federated,hsu2019measuring}.

\subsection{Deployment Limitations and Claim Boundaries}
\label{sec:supp_revision_5}

The supplementary weight-washing statistics make this mechanism concrete: the smaller $\Delta_{\text{wash}}$ of \texttt{PFAdapter} shows that preserving private $v/o$ adapters protects client-specific calibrations during aggregation, while the fairness gains in \cref{tab:supp_client_fairness} indicate that this protection benefits not only the average client but also the lower tail of the client population, a concern that is central in personalized federated learning~\cite{arivazhagan2019federated,collins2021exploiting}.

A second limitation concerns backbone scale. The present experiments are restricted to \texttt{MiniCPM-V-2\_6-int4}, so our evidence for 7B-class MLLMs is analytical rather than empirical: the synchronized payload remains tied to the selected query/key adapters, but the absolute memory footprint, optimizer state, activation storage, and local decoding/training latency still increase with backbone size. We therefore view 7B+ deployment as feasible only with additional systems support such as stronger quantization, activation checkpointing, and distributed optimizer partitioning, and we do not present the current single-GPU results as a substitute for a dedicated large-backbone study \cite{xu2025fedmllm,zhang2023federated}.

A third limitation is privacy exposure under adversarial observation. Although FL keeps raw client data local, neither vanilla LoRA aggregation nor our selective $q/k$ synchronization provides a formal defense against gradient leakage, update inversion, or membership inference attacks \cite{liu2025differentially,deng2023federated}. The server still observes transmitted adapter updates, and a malicious or compromised participant could exploit these signals to infer sensitive training attributes unless additional protection is added. We therefore frame \texttt{PFAdapter} as communication-efficient rather than intrinsically privacy-secure, and consider secure aggregation, differential privacy, and attack-aware update clipping necessary extensions for future deployment in high-risk settings.

The empirical gains are tied to their exact evidence locations: \cref{tab:main_results} shows +2.30 Acc on VQA-RAD~\cite{lau2018dataset}, +1.41 Acc on SLAKE~\cite{liu2021slake}, +3.15 AUC on Hateful Memes~\cite{kiela2020hateful}, and +1.67 Acc on CrisisMMD~\cite{alam2018crisismmd} relative to \texttt{FedYogi}, while \cref{fig:supp_sensitivity}(c) shows that the advantage increases to +3.4\% under the most heterogeneous $\alpha=0.1$ stress test. Accordingly, the revised wording replaces the earlier unsupported global 2.4\%--4.8\% range.

\begin{figure*}[t]
\centering
\includegraphics[width=\linewidth]{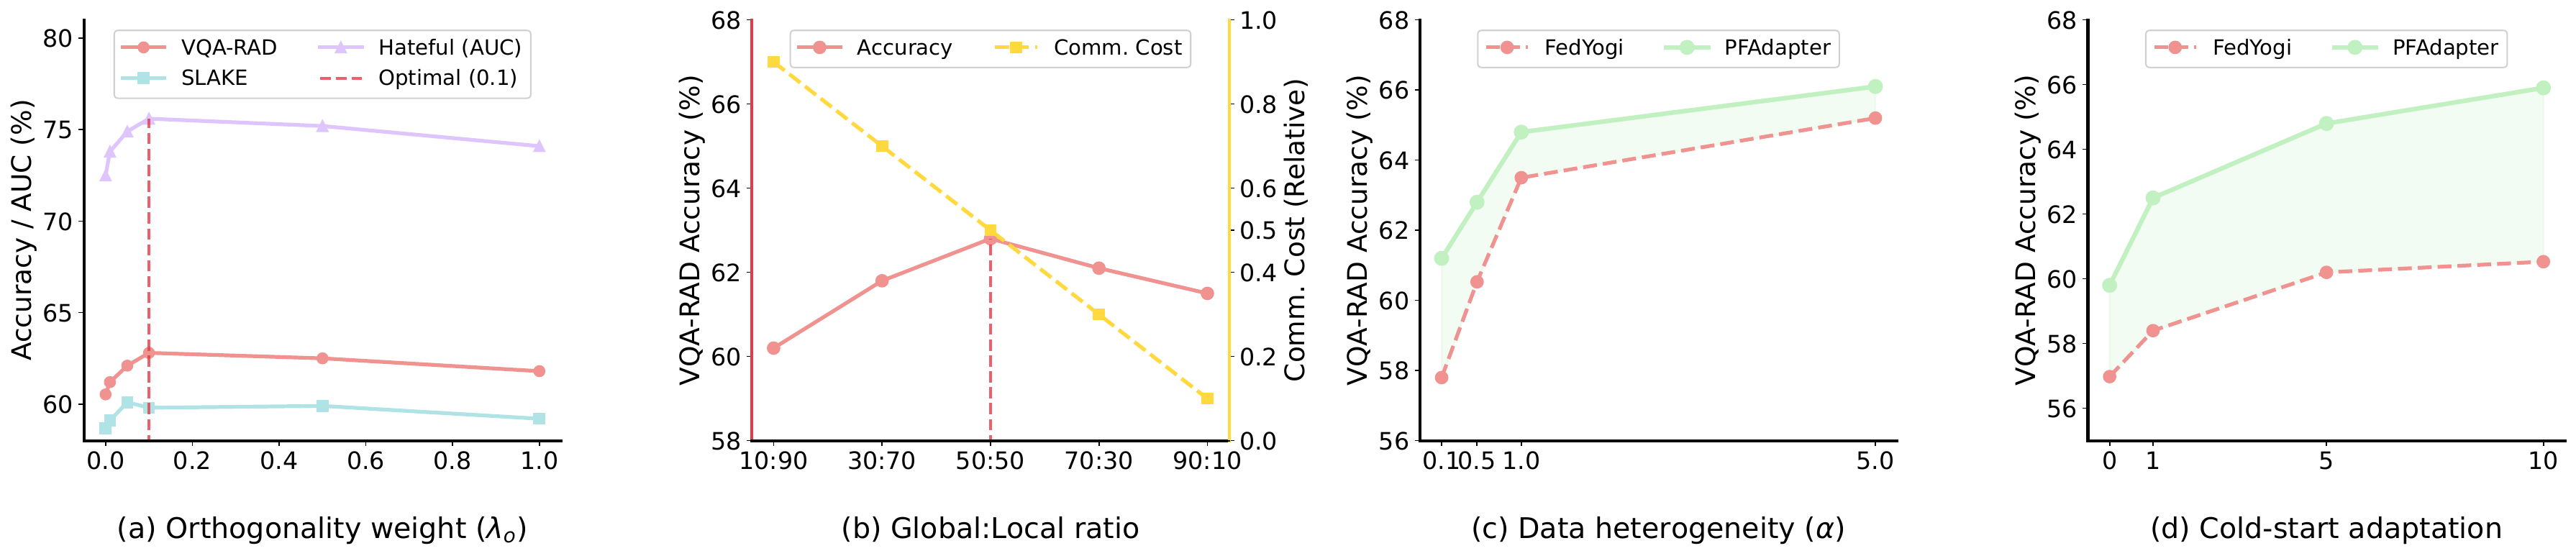}
\caption{Sensitivity analysis of \texttt{PFAdapter}. (a) Impact of orthogonality weight $\lambda_{\text{o}}$. (b) Accuracy vs. communication trade-off for decomposition ratios. (c) Robustness under data heterogeneity (Dirichlet $\alpha$). (d) Cold-start adaptation for new clients.}
\vspace{-2px}
\label{fig:supp_sensitivity}
\vspace{-10px}
\end{figure*}

\begin{table}[t]
\centering
\caption{Per-client fairness statistics on VQA-RAD.}
\vspace{-2px}
\label{tab:supp_client_fairness}
\setlength{\tabcolsep}{2.5mm}
\resizebox{\columnwidth}{!}{
\input{tbl_supp_client_fairness_body.tex}
}
\vspace{-10px}
\end{table}

\begin{table}[t]
\centering
\caption{Accuracy (\%) of heterogeneity analysis (Aligned, Missing, Cross, Hybrid scenarios) on VQA-RAD.}
\vspace{-2px}
\label{tab:supp_heterogeneity}
\setlength{\tabcolsep}{1.2mm}
\resizebox{\columnwidth}{!}{
\input{tbl_supp_heterogeneity_body.tex}
}
\vspace{-10px}
\end{table}

\begin{figure*}[t]
\centering
\includegraphics[width=\textwidth]{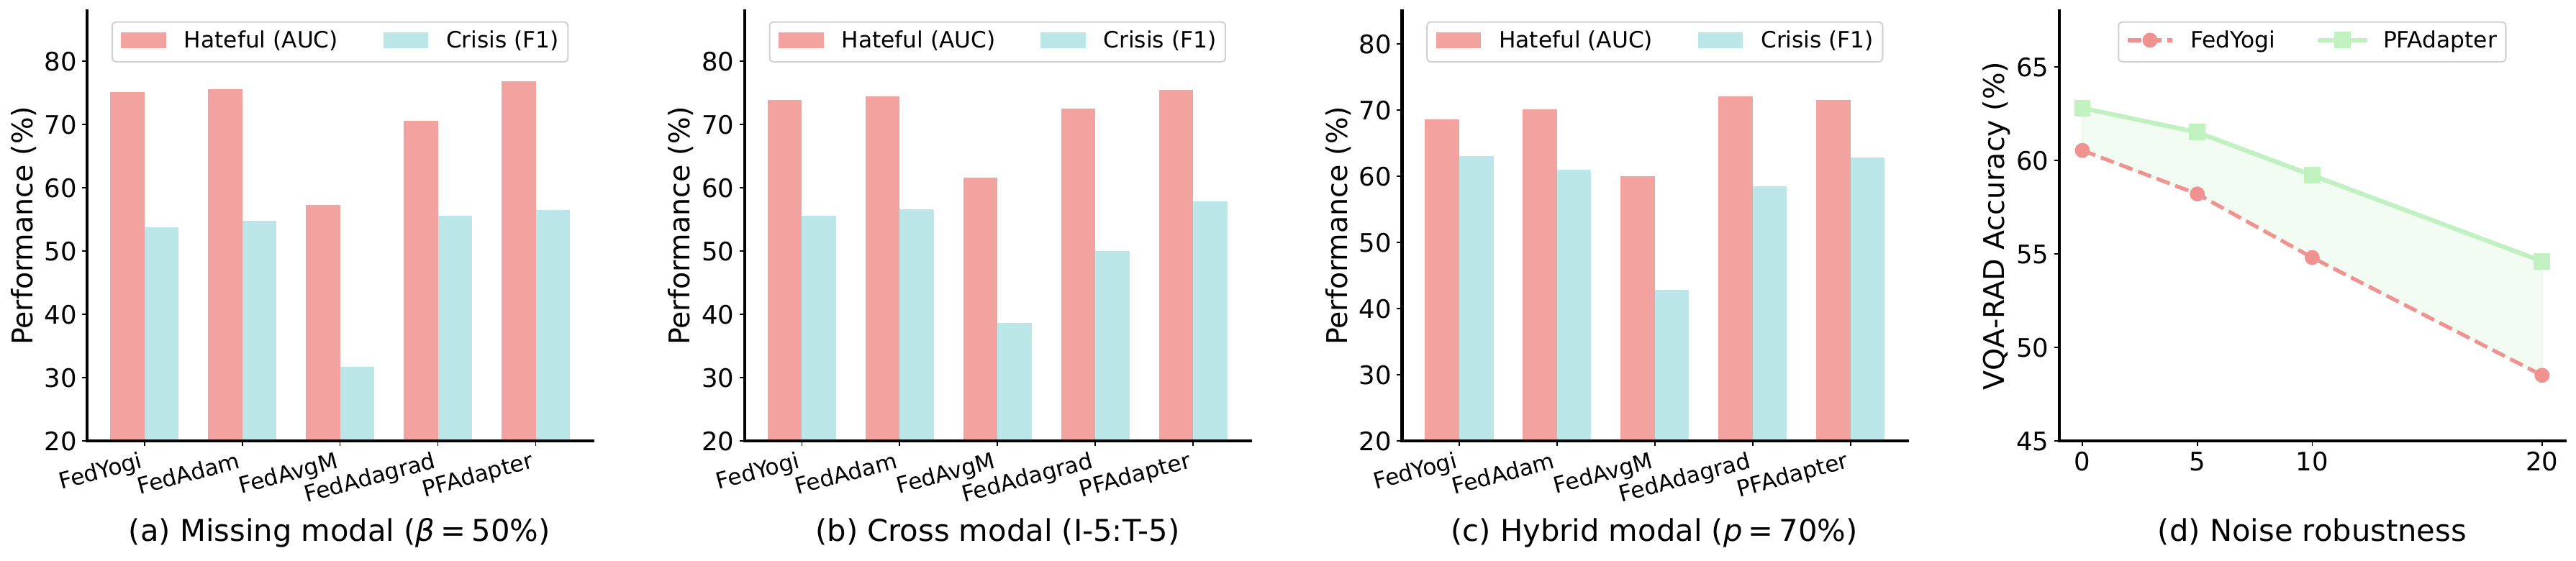}
\caption{Robustness analysis across heterogeneity scenarios, including Missing, Cross, Hybrid modalities, and noise levels.}
\vspace{-2px}
\label{fig:supp_robustness}
\vspace{-10px}
\end{figure*}

\bibliographystyle{IEEEtran}
\bibliography{refs}
\end{document}
