# Supplementary material for: PFAdapter: Hierarchical LoRA Decomposition for Personalized Federated MLLMs
Source: arXiv:2607.12111 source file (2026-10-03)
Supplement: Supplementary file 2 [file tbl_supp_attention_similarity_body.tex]

\begin{tabular}{lcccc}
\toprule
\rowcolor{gray!8}
\textbf{Projection} & $q$ & $k$ & $v$ & $o$ \\
\midrule
\textbf{Similarity} & 0.84 & 0.81 & 0.47 & 0.43 \\
\bottomrule
\end{tabular}
